# Supplementary material for: Dynamic index and LZ factorization in compressed space
Source: arXiv:1605.09558 source file (2016-07-19)
Supplement: Supplementary file 1 [file appendix_lce_hconstruction.tex]

%\section*{Appendix B : Theorem~\ref{theo:HConstructuionTheorem}}
\section{Appendix: Omitted Proofs in Section~\ref{sec:Construction}}\label{sec:Proof_HConstructuionTheorem}

\subsection{Proof of Theorem~\ref{theo:HConstructuionTheorem}~(2)}
\begin{proof}
\tnnote*{modified}{
	%Consider $\mathcal{H}(f_{\mathcal{A}}, f'_{\mathcal{A}})$ for an empty signature encodings $\mathcal{G}$. 
	Consider a dynamic signature encoding $\mathcal{G}$ for an empty string. 
	%If we can compute $\mathit{INSERT}(Y,i)$ operation in $O(f_{\mathcal{A}}\log N \log^* M)$ time, 
	Then Theorem~\ref{theo:HConstructuionTheorem}~(2) immediately holds 
	by computing $\mathit{INSERT'}(c_i,|f_i|,|f_1 \cdots f_{i-1}|+1)$ for all $1 \leq i \leq z$ incrementally, 
	where $c_i \leq |f_1 \cdots f_{i-1}| - |f_i|$ is a position such that $T[c_i..c_i+|f_i|-1] = f_i$ holds.
	%By the proof of Lemma~\ref{lem:INSERT_DELETE}, 
	%we can compute $\mathit{INSERT}(Y,i)$ for a given $\uniq{Y}$ in $O(f_{\mathcal{A}}\log N \log^* M)$ time. 	
	%We can compute each $\uniq{f_i}$ in $O(\log N \log^* M)$ time by Lemma~\ref{lem:ComputeShortCommonSequence} 
	%because $f_i$ occurs previously in $T$ when $|f_i| > 1$. 
	%Hence we get Theorem~\ref{theo:HConstructuionTheorem}~(2).	
	%Note that we can compute $\mathit{Uniq}(f_i)$ in $O(\log N \log^* M)$ time by Lemma~\ref{lem:ComputeShortCommonSequence}
	%because $f_i$ is a substring of $f_1 \cdots f_{i-1}$ when $|f_i| > 1$.
	%Hence $\mathit{INSERT}(f_i,|f_1 \cdots f_{i-1}|)$ can be computed in $O(f_{\mathcal{A}} \log N \log^* M)$ time 
	%by Lemma~\ref{lem:INSERT_DELETE}.
	%Therefore Theorem~\ref{theo:HConstructuionTheorem}~(2) holds. 
	% \qed
}
\end{proof}
Note that we can directly show Lemma~\ref{lem:upperbound_signature} from the above proof 
because the size of $\mathcal{G}$ increases $O(\log N \log^* M)$ by Lemma~\ref{lem:ancestors}, 
every time we do $\mathit{INSERT'}(c_i,|f_i|,|f_1 \cdots f_{i-1}|+1)$ for $1 \leq i \leq z$.

\subsection{Proof of Theorem~\ref{theo:HConstructuionTheorem}~(3a)}
\begin{proof}
	%We can construct $\mathcal{H}(f_{\mathcal{A}},f'_{\mathcal{A}})$ by $O(n)$ $\mathit{INSERT}$ operations 
	We can construct the dynamic signature encoding $\mathcal{G}$ for $T$ by $O(n)$ $\mathit{INSERT'}$ operations 
	as the proof of Theorem~\ref{theo:HConstructuionTheorem}~(2).
\end{proof}

\subsection{Proof of Lemma~\ref{lem:Lambda_t}}\label{sec:Proof_Lambda_t}
\begin{proof}
We first compute, for all variables $X_i$,
$\encpow{\xshrink{t}{X_i}}$ if $|\encpow{\xshrink{t}{X_i}}| \leq \Delta_{L} + \Delta_{R} + 9$,
otherwise $\encpow{\hat{L}_{t}^{X_i}}$ and $\encpow{\hat{R}_{t}^{X_i}}$.
The information can be computed in $O(n \log^*M)$ time and space in a bottom-up manner, i.e., by processing variables in increasing order.
For $X_i \rightarrow X_{\ell} X_{r}$, if both $|\encpow{\xshrink{t}{X_{\ell}}}|$ and $|\encpow{\xshrink{t}{X_{r}}}|$ are no greater than $\Delta_{L} + \Delta_{R} + 9$,
we can compute $\encpow{\xshrink{0}{X_i}}$ in $O(\log^* M)$ time 
by naively concatenating $\encpow{\xshrink{t}{X_{\ell}}}$, $\encpow{\hat{z}_{t}^{X_i}}$ and $\encpow{\xshrink{t}{X_{r}}}$.
Otherwise $|\encpow{\xshrink{t}{X_i}}| > \Delta_{L} + \Delta_{R} + 9$ must hold, and 
$\encpow{\hat{L}_{0}^{X_i}}$ and $\encpow{\hat{R}_{0}^{X_i}}$ can be computed in $O(1)$ time from $\encpow{\hat{z}_{t}^{X_i}}$ and the information for $X_{\ell}$ and $X_{r}$.

The run-length encoded signatures represented by $z_{t}^{X_i}$ can be obtained in $O(\log^* M)$ time
by using $\hat{z}_{t}^{X_i}$ and the above information for $X_{\ell}$ and $X_r$:
$z_{t}^{X_i}$ is created over run-length encoded signatures that are obtained by concatenating 
$\encpow{\xshrink{0}{X_{\ell}}}$ (or $\encpow{\hat{R}_{0}^{X_{\ell}}}$), $z_{t}^{X_i}$ and $\encpow{\xshrink{0}{X_r}}$ (or $\encpow{\hat{R}_{0}^{X_r}}$).
Also, $A_{t}^{X_n}$ and $B_{t}^{X_n}$ represents $\hat{A}_{t}^{X_n} \hat{L}_{t}^{X_n}$ and $\hat{R}_{t}^{X_n} \hat{B}_{t}^{X_n}$, respectively.

Hence, we can compute in $O(n \log^* M)$ time $O(n \log^*M)$ run-length encoded signatures to which we give signatures.
We determine signatures in $O(n \log \log n \log^* M)$ time by sorting the run-length encoded signatures as Lemma~\ref{lem:Lambda_t}.
\end{proof}
