# Supplementary material for: Dynamic index and LZ factorization in compressed space
Source: arXiv:1605.09558 source file (2016-07-19)
Supplement: Supplementary file 2 [file appendix_proof_update.tex]

%\section{Appendix: Proof of Lemma~\ref{lem:INSERT_DELETE}}\label{sec:appendix_proof_update}
%\begin{proof}
%Let $\mathcal{G} = (\Sigma, \mathcal{V}, \mathcal{D}, S)$ be the signature encoding before the update operation.
%
%We support $\mathit{DELETE}(i,k)$ as follows:
%(1) Compute a new start variable $S' = \id{T[..i-1]T[i..]}$ 
%by recomputing the new signature encoding from $\mathit{Uniq}(T[..i-1])$ and $\mathit{Uniq}(T[i+k..])$.
%This can be done in $O(f_{\mathcal{A}}\log N \log^* M)$ time 
%by Lemmas~\ref{lem:ComputeShortCommonSequence} and \ref{lem:ancestors}. 
%(2) Remove all redundant signatures $Z$ from the dynamic $\mathcal{H}$.
%Note that if a signature is redundant, then all the signatures along the path from $S$ to it are also redundant.
%Hence, we can remove all redundant signatures efficiently by depth-first search starting from $S$,
%which takes $O(f_{\mathcal{A}}|Z|)$ time, where $|Z| = O(k + \log N \log^* M)$ by Lemma~\ref{lem:ancestors}.
%
%Similarly, we can compute $\mathit{INSERT}$ operation in $O(f_{\mathcal{A}}(|Y| + \log N \log^* M))$ time 
%by creating $S'$ using $\mathit{Uniq}(T[..i-1])$, $\mathit{Uniq}(Y)$ and $\mathit{Uniq}(T[i+k..])$. 
%Note that we can naively compute $\id{s}$ for a given string $s \in \Sigma^+$ in $O(f_{\mathcal{A}} |s|)$ time. 
%Therefore Lemma~\ref{lem:INSERT_DELETE} holds.
%%%%\qed
%\end{proof}
